# Supplementary material for: MiniCLEAN Dark Matter Experiment
Source: arXiv:1711.02117 source file (2017-11-06)

Chris Benson  
6/9/2015

# Magnetic Field sensor orientations.

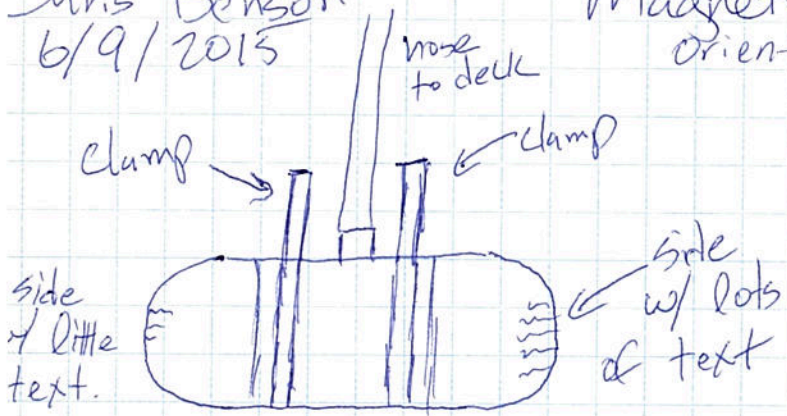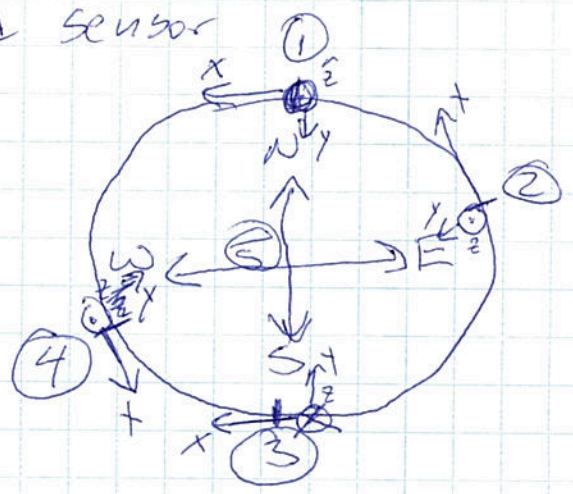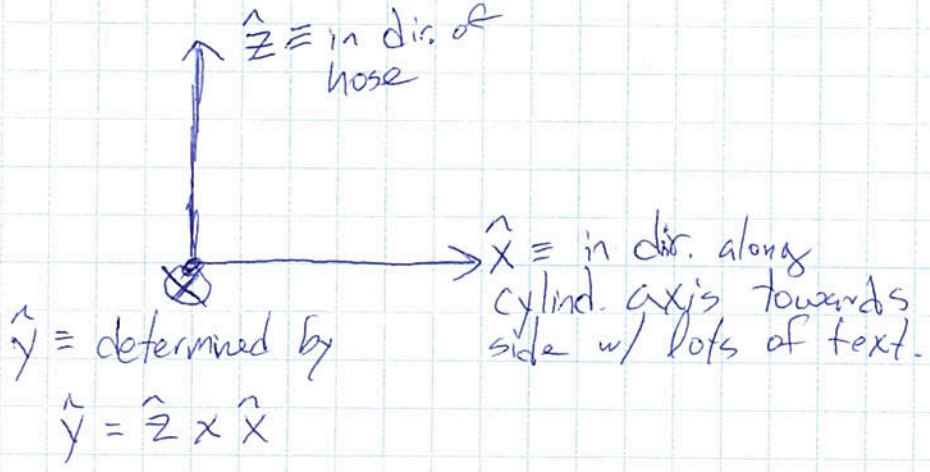

## Sensor orientation and position

① North sensor: Hanging on OV-S, 3° East of North.

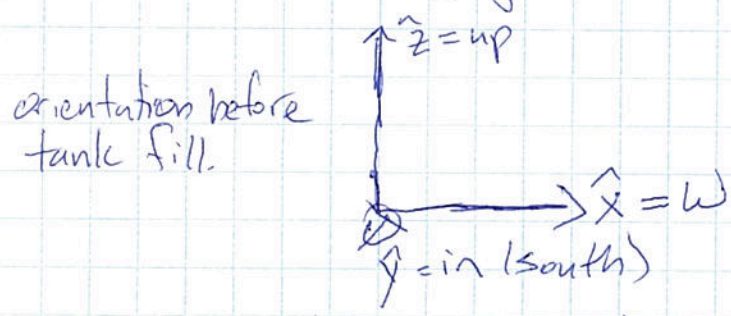

② East sensor: Hanging on OV-R, 15° North of East.

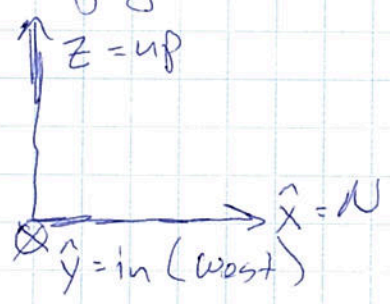

③ South sensor - Hanging on OV-L,  $3^\circ$  West of South

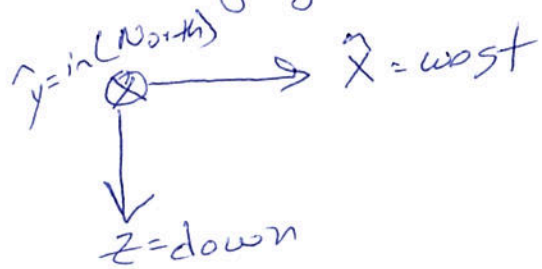

④ West Sensor - Hanging on OV-K,  $15^\circ$  South of W.

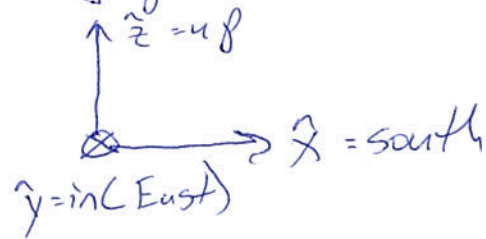

⑤ Top Sensor - Hanging Above OV on center.  
pointing North

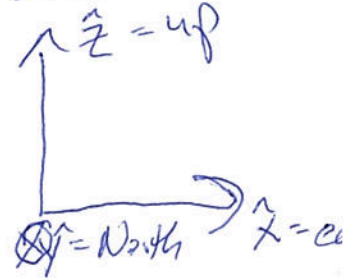

Supplement: Supplementary file 1 [file mag_sensor_location.pdf]
